# Supplementary material for: Bias Beyond English: Counterfactual Tests for Bias in Sentiment Analysis in Four Languages
Source: arXiv:2305.11673 source file (2023-05-19)
Supplement: Supplementary file 1 [file all_confusion_appendix.tex]

\begin{figure*}[ht]
    \centering
    \begin{subfigure}[b]{\textwidth}
        \includegraphics[width=\textwidth]{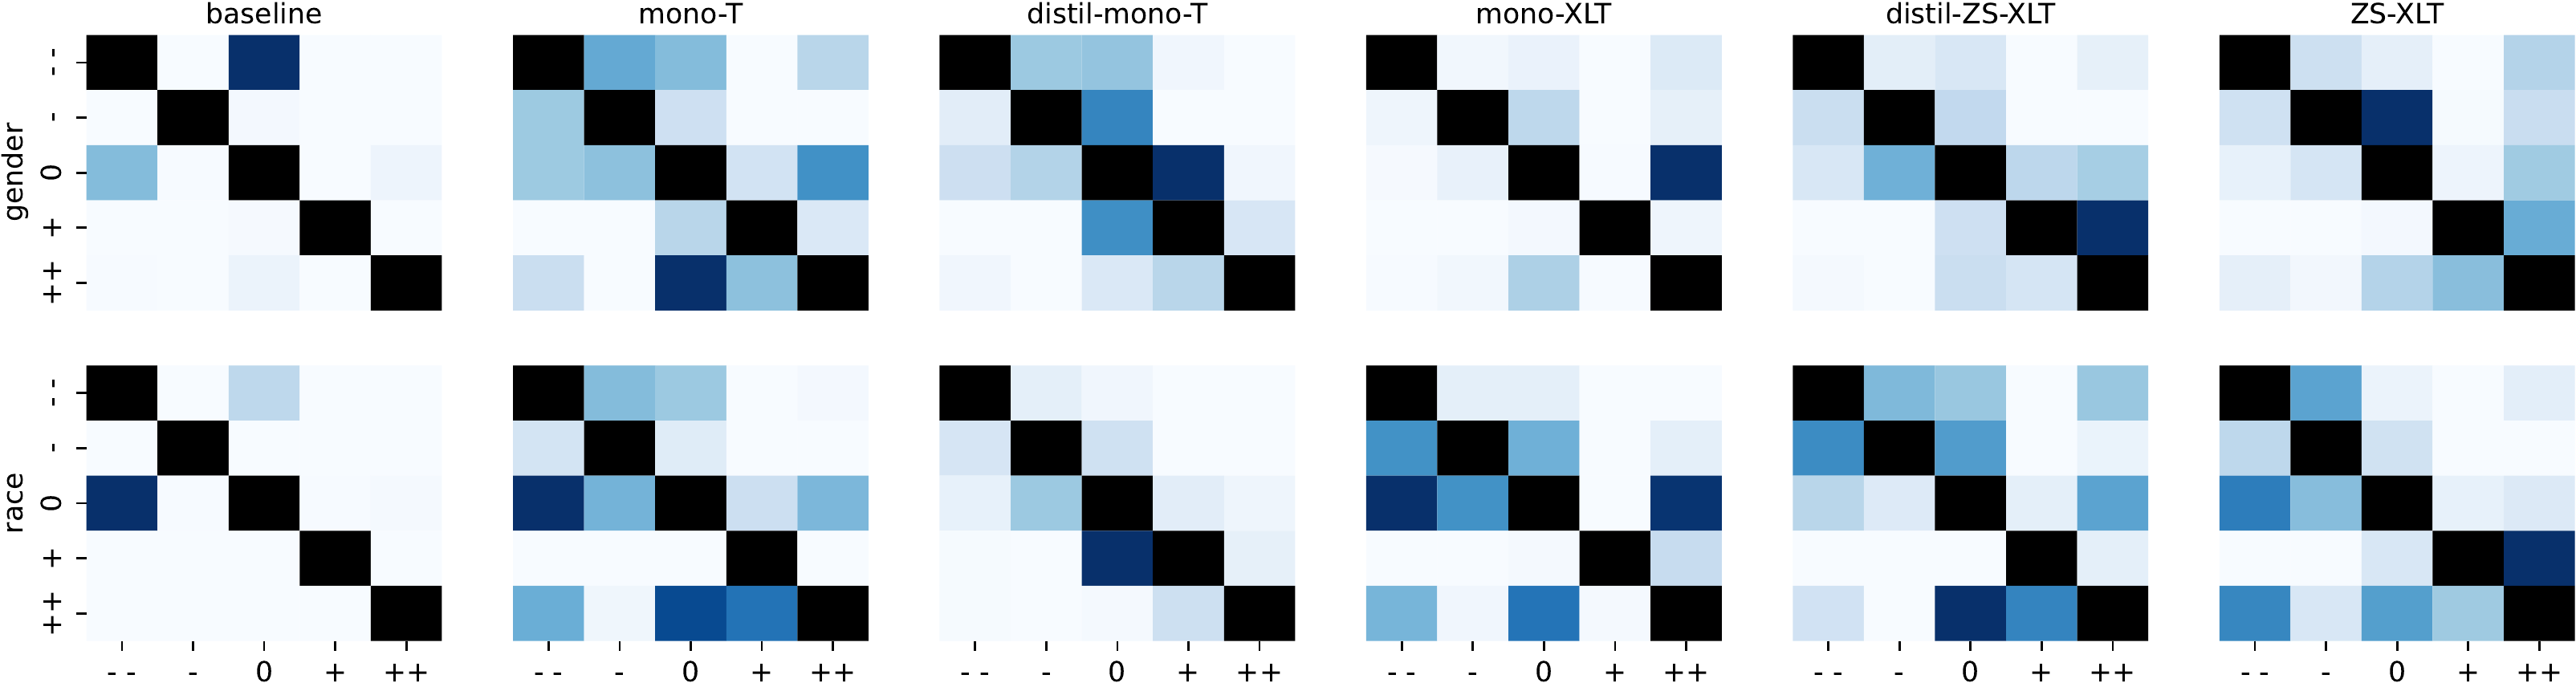}
        \caption{Japanese (ja)}
        \label{fig:b}
    \end{subfigure}
    ~
    \begin{subfigure}[b]{\textwidth}
        \includegraphics[width=\textwidth]{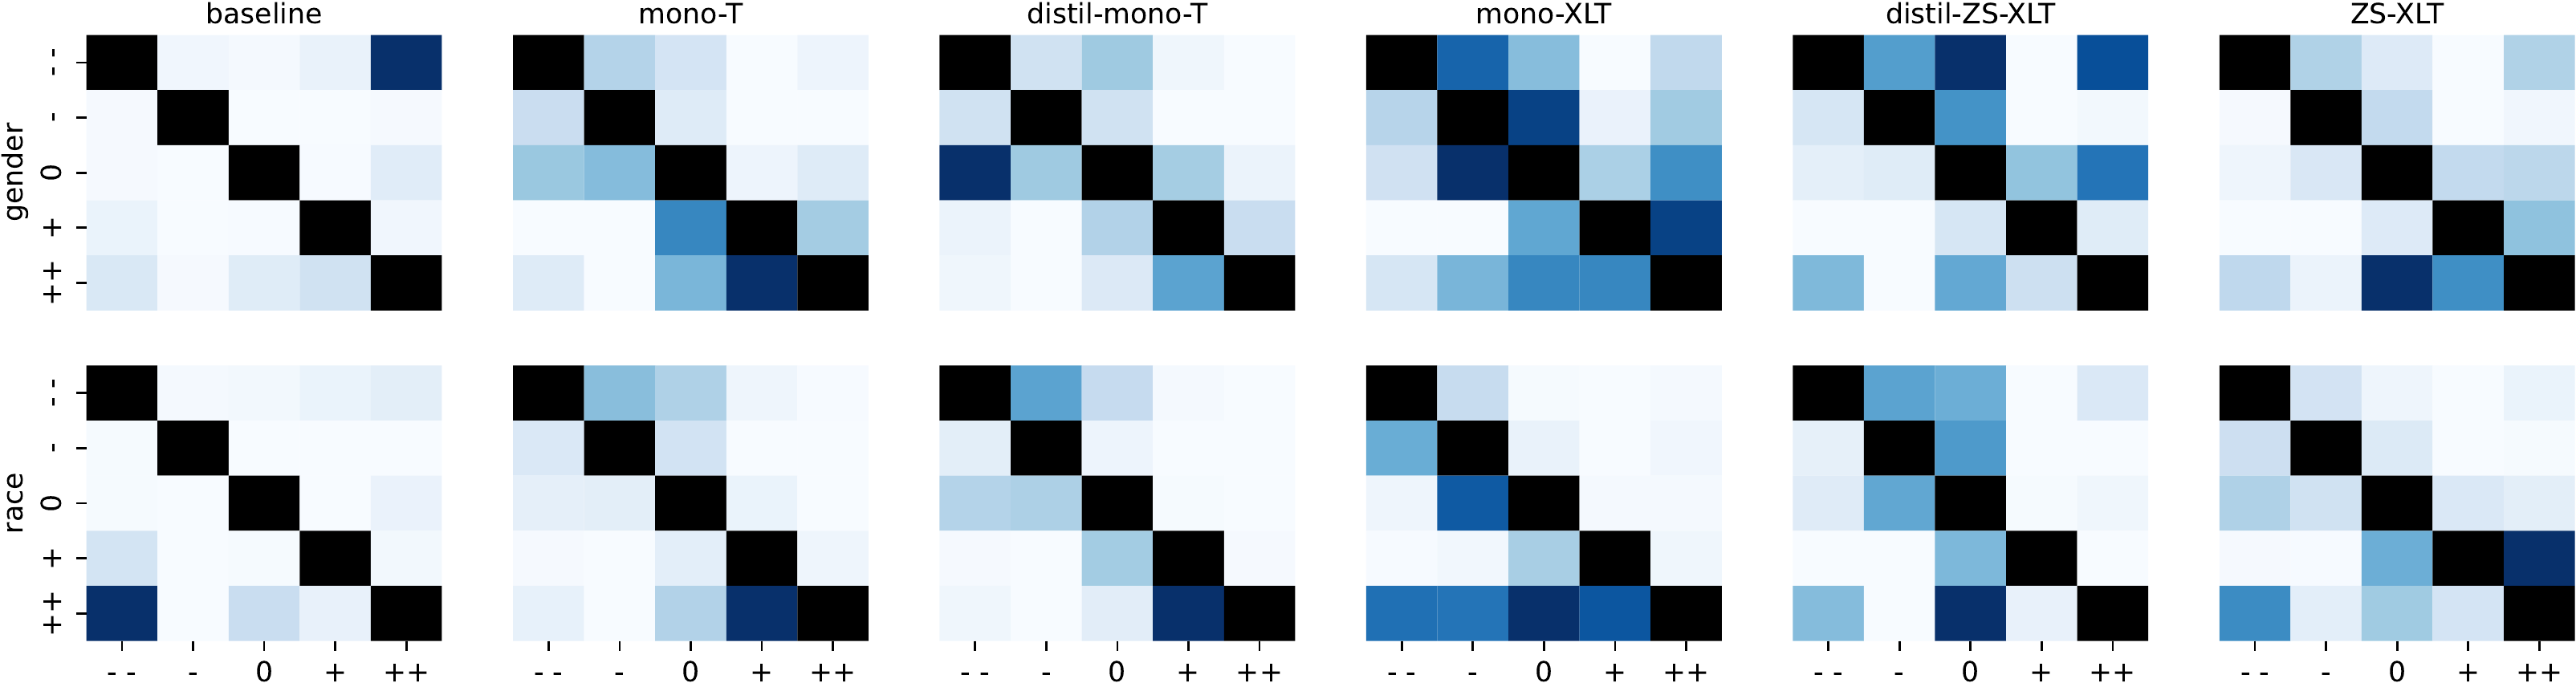}
        \caption{German (de)}
        \label{fig:}
    \end{subfigure}
    ~ 
    \begin{subfigure}[b]{\textwidth}
        \includegraphics[width=\textwidth]{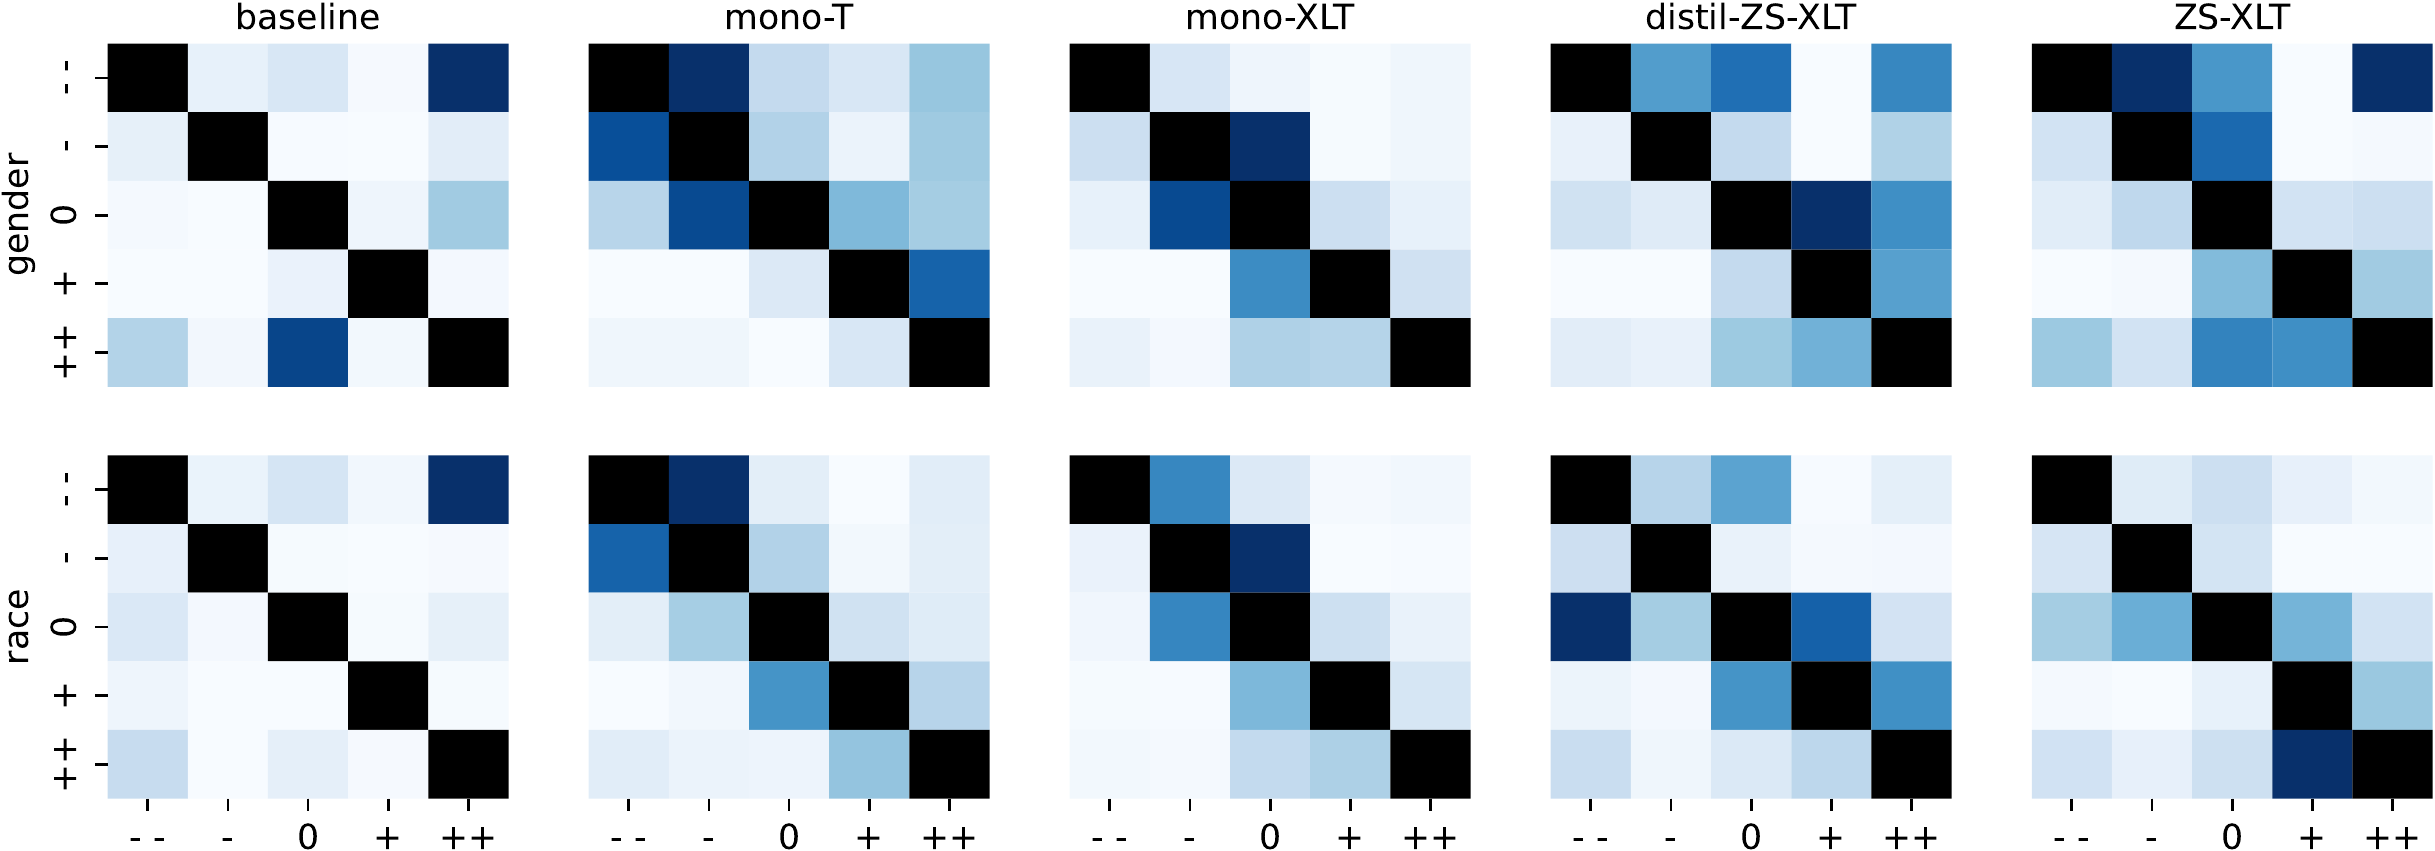}
        \caption{Spanish (es)}
        \label{fig:}
    \end{subfigure}
    ~ 
    \begin{subfigure}[b]{\textwidth}
        \includegraphics[width=\textwidth]{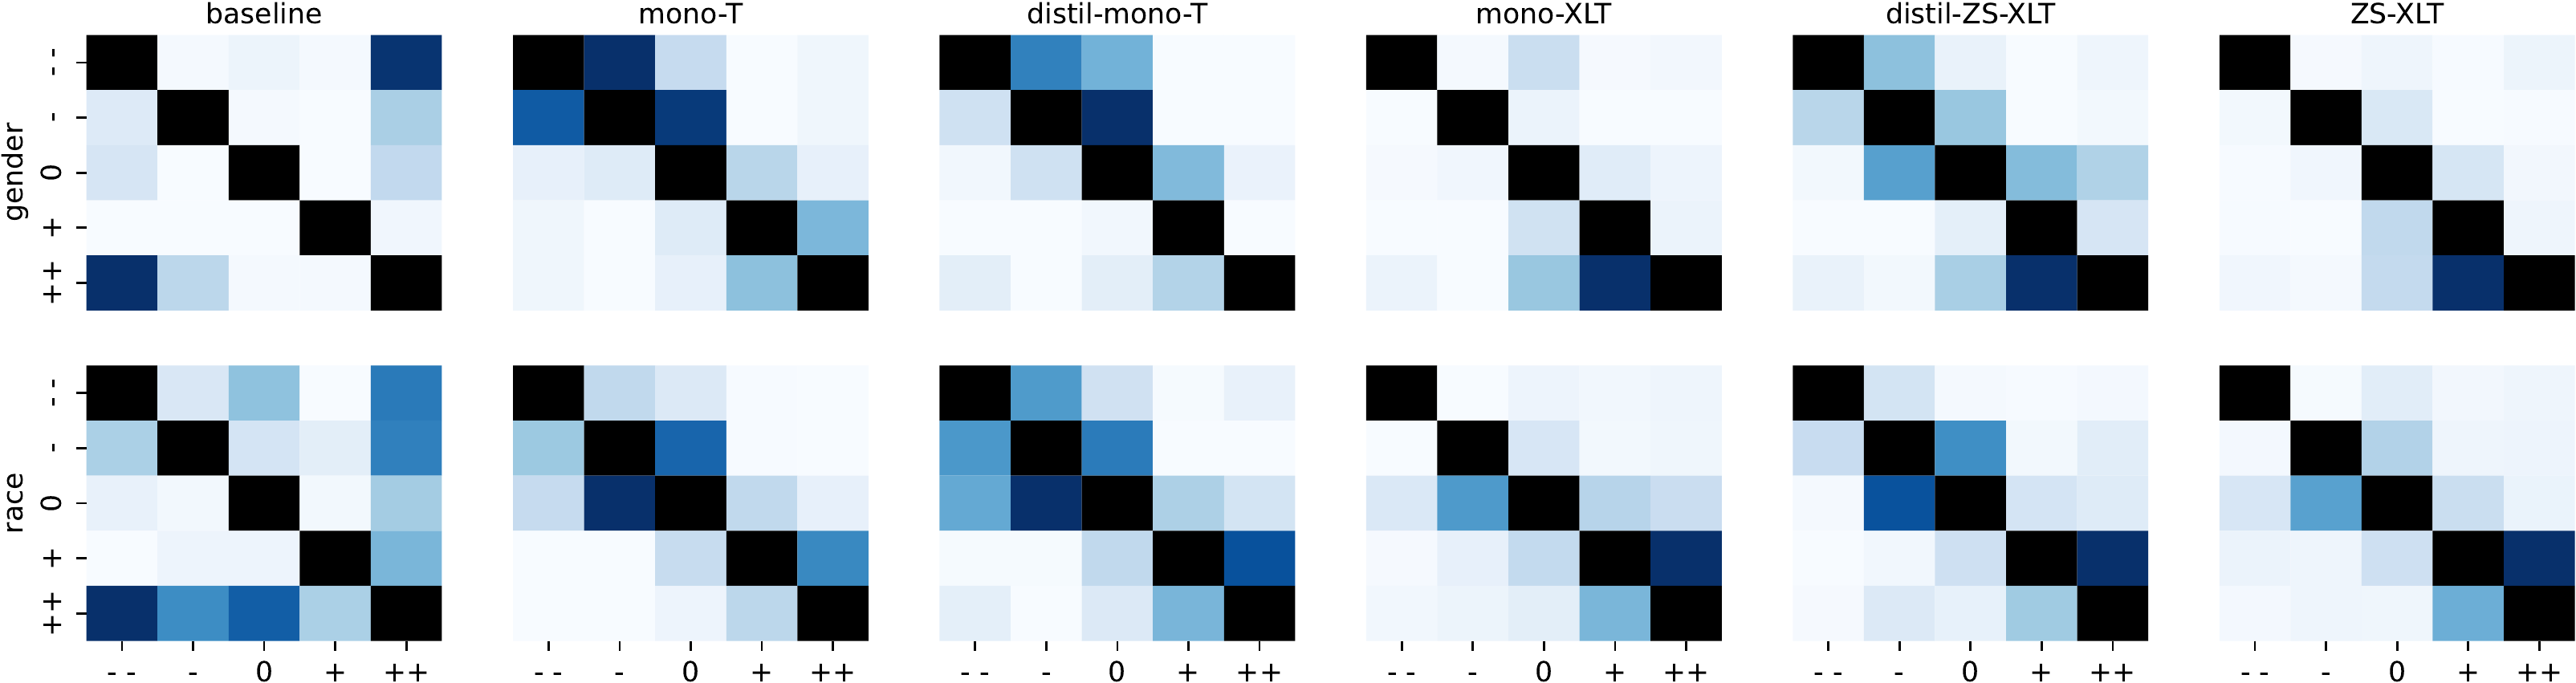}
        \caption{English (en)}
        \label{fig:}
    \end{subfigure}
    ~
    \begin{subfigure}[b]{\textwidth}
        \includegraphics[width=\textwidth]{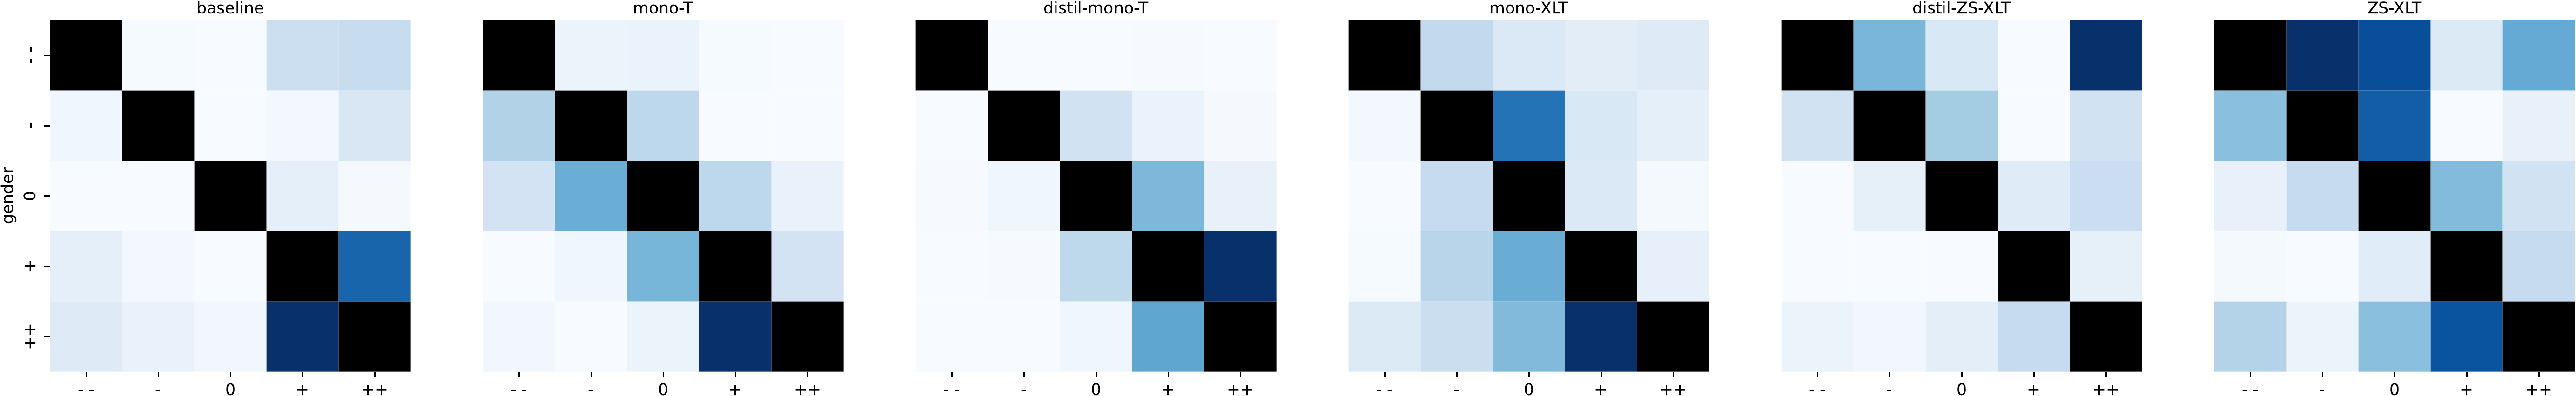}
        \caption{Chinese (zh\_cn)}
        \label{fig:}
    \end{subfigure}
    \caption{All confusion matrices for experiments in this paper. \textbf{++} to \textbf{-{}-} are sentiment scores. Rows are predicted sentiment scores for the privileged group, columns predicted scores for the minoritised group. Higher colour saturation in the lower triangle is therefore bias against the minoritised group, in the upper triangle is bias against the privileged group.} 
    \label{fig:all_confusion}
\end{figure*}
